# Supplementary material for: Extremal combinatorics, iterated pigeonhole arguments, and generalizations of PPP
Source: arXiv:2209.07625 source file (2022-09-15)
Supplement: Supplementary file 1 [file appendixExp.tex]

\subsection{k-Value Long Choice}

Above, we have defined a family of Ramsey problems ($(r,n)$-Ramsey) based on the number of colors we use to color the edges of a complete graph. In similar vein, we can define a sequence of Long Choice problems in which the predicates can take on $k\geq{2}$ values (as opposed to only $2$). 

\begin{defi}[$k$-value Long Choice]
	Consider a set $S$ of $2^n$ objects, $\{a_i\}$, each represented by a unique binary $n$-bit string, where $n > log(k)$. We are given a sequence of $t = 1 + \lceil \log_{k} (2^n - 1) \rceil$ predicate functions, $P_0, \dots, P_{t-1}$. Predicate function $P_i$ has arity $i + 1$: 
	$$ P_i : S^{i+1} \mapsto \{0,1,\dots k\}$$
	The $P_i$ are concisely represented. We are also given an initial element $a_0$. The problem is to find any of the following:
	\begin{enumerate}
		\item \textbf{Long Choice: }A sequence of $n+1$ points in $S$, $a_0, \dots, a_{n}$, with the following property: for all $i$ in $[0, \dots, n-1]$, for all $j > i$, $P_i(a_0, \dots, a_{i},a_{j})$ is constant.
		\item \textbf{Error: }A sequence of points $a_0, \dots, a_i, a_j$ with $P_i(a_0, \dots, a_i, a_j) = k$.
	\end{enumerate}
\end{defi}

Note that in the above problem, $n > log(k)$. We now prove a completeness result related to PPP. 

\begin{theorem}
	$(2^{n} - 2)$-value Long Choice is PPP-complete
\end{theorem}

\begin{proof}
	We begin by proving that $2^{n} - 2$-value Long Choice is PPP-hard. We start with an instance of a PPP-complete problem, Pigeonhole Circuit. We are given a circuit, $C$, mapping $n$-bit strings to $n$-bit strings: 
	
	$$C: \{0,1\}^{n}  \mapsto \{0,1\}^n$$
	
	The challenge, as usual, is to find two distinct $n$-bit strings $x$ and $y$ with $C(x) = C(y)$ or find a $n$-bit string $z$ with $C(z) = 0$. For the rest of this discussion, we refer to the $n$-bit string using its corresponding decimal value. For example, the string $0^n$ is $0$. 
	
	We accordingly define a $2^{n} - 2$-value Long Choice problem instance. This problem instance has $2$ predicate functions, $P_0$ and $P_1$. There are $2^n$ objects in this problem instance, each encoded in the standard way by an $n$-bit string. As above, we will refer to these objects using the decimal value of their binary encodings. For brevity, instead of saying `object $2$', we will just say $2$. 
	
	We let our initial object $a_0$ be $1$. If $C(1) = 0$, then we are done. Otherwise, we define a value $j$ to be $1$ if $C(1)\neq{1}$, and $2$ otherwise. We now define a new, modified circuit, $C'$ with the same domain and range as $C$. On input $i$, $C'(i)$ is defined based on the following cases: 
	\begin{enumerate}
		\item If $C(i) = 0$ or $C(i) = C(1)$, then $C'(i) = j$. 
		\item Otherwise, $C'(i) = C(i)$
	\end{enumerate}

	In the modified circuit $C'$, no element maps to $0$, and no elements map to $C(1)$, based on the above definition. Thus, there are at most $2^n - 2$ values which $C'$ can take. These values fall in the set $\{1, 2, \dots, 2^n - 1\}\setminus(C(1))$. 
	
	Finally, we define the predicate functions $P_0$ and $P_1$.	$P_0(a_0, a_1)$ can take any value from the set $\{0, 1, \dots, 2^n - 2\}$. It has an output that depends solely on $C'(a_1)$. Specifically, $P_0(a_0, a_1)$ is: 
	
	\begin{enumerate}
		\item $C'(a_1) - 2$ if $C'(a_j) > C(1)$. 
		\item $C'(a_1) - 1$ otherwise
	\end{enumerate}
	
	$P_1(a_0, a_1, a_2)$ unconditionally outputs $1$ (in other words, it is unimportant to this reduction). 
	
	Consider a certificate to this problem, consisting of $3$ objects, $a_0, a_1, a_2$. By the definition of $k$-Value Long Choice, we know that $P_0(a_0, a_1) = 	P_0(a_0, a_2)$. This, in turn, means that $C'(a_1) = C'(a_2)$. To see why, suppose that $C'(a_1) \neq{C'(a_2)}$. Then, one of these values must be greater than $C(1)$, and the other must be less than $C(1)$. Suppose, without loss of generality, that $C'(a_1) > C(1)$ and $C'(a_2) < C(1)$. Then $P_0(a_0, a_1)  = C'(a_1) - 2  > C'(a_2) - 1 = P_0(a_0, a_2)$, so $P_0(a_0, a_1) \neq{P_0(a_0, a_2)}$. 
	
	If $C'(a_1) = C'(a_2)$, then we have two cases to consider. First, if either $C(a_1)$ or $C(a_2)$ are zero, we are done. If either $C(a_1)$ or $C(a_2)$ are equal to $C(1) = C(a_0)$, then we have found a collision. Otherwise, we note that $C'(a_1) = C'(a_2) = C(a_1) = C(a_2)$ and we have found a collision. In any case, we have found a certificate to the original problem.

	Now we prove that $(2^n - 2)$-value Long Choice is in PPP. To do so, consider any instance of $(2^n - 2)$-value Long Choice. This is defined by the predicate functions $P_0$ and $P_1$. We are also given an initial element $a_0$. Note that to find a suitable Long Choice certificate, it suffices to find two distinct elements $a_1$ and $a_2$, with $P_0(a_0, a_1) = P_0(a_0, a_2)$. As mentioned above, $P_1$ is irrelevant. The predicate function $P_0$ takes values in the set $\{0, 1, \dots, 2^n - 3\}$ (there are no errors, so the predicate functions never output $2^n - 2$). We now define a Pigeonhole Circuit, $C$, which maps $n$-bit strings to $n$-bit strings, as follows. Each $n$-bit string in the domain of $C$ refers to an object from the Long Choice problem instance. So, conceptually, $C$ takes, as input, an object $a_i$. The output $C(a_i)$ is:
	
	\begin{enumerate}
		\item $P_0(a_0, a_i) + 1$ if $a_i\neq{a_0}$
		\item $2^n - 1$ otherwise
	\end{enumerate}

	Note that in this mapping, no element is mapped to $0$. However, there are $2^n$ objects, and $2^n - 1$ possible values which they can take under the mapping, $C$. Thus, there must be two distinct objects which take the same value. Furthermore, neither of these objects can be $a_0$ based on the above definition. Therefore, there are two distinct values $a_i$ and $a_j$, neither of which are $a_0$ with the property that $C(a_i) = C(a_j)$. This in turn means that $P_0(a_0, a_i) = P_0(a_0, a_j)$. Thus, $P_0(a_0, a_i, a_j)$ forms a valid Long Choice certificate. 
\end{proof}

Above, we proved that $(r, n)$-Ramsey reduces to Long Choice, for all $r > 2$. Using the exact same argument, we see that $(r,n)$-Ramsey reduces to $r$-value Long Choice. 

\begin{theorem}
	$(r,n)$-Ramsey reduces to $r$-value Long Choice
\end{theorem}

\begin{proof}
	We prove this result in the case that $r$ is a power of $2$, noting that it generalizes to other values of $r$ as well. Suppose $r = 2^m$. Then the $(r,n)$-Ramsey problem asks: given a complete graph of $r^{rn} = 2^{r*log(r)*n}$ vertices whose edges are each colored one of $r$ colors, find a monochromatic clique. Consider the proof (discussed above) that this problem is a total problem. It involves constructing a sequence of vertices $a_0, a_1, \dots, a_{rn}$ with the property that for any $i$, $(a_i, a_j)$ and $(a_i, a_k)$ both have the same color whenever $i < j, k$. Using this sequence, the proof then finds a monochromatic clique by applying the Pigeonhole Principle. The key point here is that $a_0, a_1, \dots, a_{rn}$ is a Long Choice sequence. The predicate functions are clear: $P_0(a_0, a_i)$ outputs the color between edge $(a_0, a_i)$. More generally, $P_x(a_0, a_1, \dots, a_x, a_i)$ outputs the color between vertex $a_x$ and $a_i$. Thus, given an instance of $(r,n)$-Ramsey problem, we construct a $r$-value Long Choice problem instance with $2^{rlog(r)*n}$ objects, with the predicate functions defined as above. Any solution to this problem will yield a clique. 
\end{proof}
